# Supplementary material for: An Optimal Algorithm for Higher-Order Voronoi Diagrams in the Plane: The Usefulness of Nondeterminism
Source: arXiv:2310.15363 source file (2023-10-23)
Supplement: Supplementary file 1 [file appendices.tex]

\begin{appendices}

\section{Solving Recurrence Relation in~\Cref{eq:rr}}
\label{sec:solve-rr}
We have the following recurrence relation~\Cref{eq:rr}
\[
    T(n,m)=T(n_1,m_1)+T(n_2,m_2)+O((n+\sqrt{m})\log^6(n+\sqrt{m})),
\]
where $n_1+n_2\le n$, $m_1+m_2 \le m$, and $m_1,m_2\le 2\sqrt{2m}$.

Let $N$ and $M$ be the number of planes and the size of the $k$-level in the beginning.
Consider nodes with $b\le m\le 2b$ where $b=2^i$ for $i=0,1,\cdots,\log (M/2)$
in the recursion tree of Equation~\Cref{eq:rr}.
The number of such nodes is bounded by $M/b$.
Then to bound the total cost of nodes with $m$ in this range, 
it suffices to bound
\[
    \sum_{i} (n_i+\sqrt{b})\log(n_i+\sqrt{b}),
\]
where $n_i$ is the number of the corresponding number of planes assigned to the problem
and $\sum_i n_i = N$.

Note that
\begin{align*}
    \sum_{i} (n_i+\sqrt{b})\log^6(n_i+\sqrt{b})
    &\le \sum_{i} (n_i+\sqrt{b})(\log^6 n_i+\log^6b) \\
    &= \sum_{i} n_i\log^6n_i + \sqrt{b}\log^6n_i + n_i\log^6b + \sqrt{b}\log^6b \\
    &\le N\log^6N + N\log^6b + \frac{M}{\sqrt{b}}\log^6b + \sqrt{b} \sum_{i} \log^6n_i \\
    &\le c N\log^6N + \frac{M}{\sqrt{b}} \log^6\frac{Nb}{M} \\
    &\le c (N\log^6N + \frac{M\log^6b}{\sqrt{b}}),
\end{align*}
where the third last inequality follows from the total number of such nodes is at most $M/b$,
the second inequality follows from Jensen's inequality,
and the last inequality follows from $M = Nk$.

Thus the total running time is bounded by summing over all nodes of size $b$:
\[
    \sum_b c\left(N\log^6N+\frac{M\log^6b}{\sqrt{b}}\right)
    = \sum_{i=1}^{\log(M/2)} c\left(N\log^6 N+\frac{Mi^6}{2^{i/2}}\right) = O(N\log^{O(1)}N + M).
\]

This proves that $T(n, m)=O(n\log^{O(1)}n + m)$.

\end{appendices}
